# Supplementary material for: Viscosity of protein-stabilised emulsions: contributions of components and development of a semi-predictive model
Source: arXiv:1810.03905 source file (2018-10-09)
Supplement: Supplementary file 1 [file SupplementaryMaterial.pdf]

# Supplementary material for: Viscosity of protein-stabilised emulsions: contributions of components and development of a semi-predictive model

Marion Roullet, Paul S. Clegg, William J. Frith

September 24, 2018

## 1 Error bars

The error bars indicated in the figures indicates the uncertainty of the measurements and/or the calculations, and are calculated using the error propagation theory that we shortly describe here. More information can be found in P. Fornasini *The Uncertainty in Physical Measurements*, Springer 2008, Chapter 8.

The uncertainty of each quantity is calculated from the uncertainty of its variables, assuming that these are independent. In practice, if the quantity $R$ is calculated as a function of quantities $X$, $Y$, $Z\ldots$- assumed to be independent - and if each one of those presents an uncertainty $\delta X$, $\delta Y$, $\delta Z\ldots$; then the uncertainty $\delta R$ can be written:

$$\delta R = \sqrt{\left(\frac{\partial R}{\partial X} \times \delta X\right)^2 + \left(\frac{\partial R}{\partial Y} \times \delta Y\right)^2 + \left(\frac{\partial R}{\partial Z} \times \delta Z\right)^2 + \ldots} \tag{1}$$

Here, the calculations for the uncertainty were performed for each quantity calculated, using either the uncertainties derived previously, or the standard errors obtained from the fitting procedure or from the calculation of the mean value. The resulting uncertainty is not a standard error in the strict statistical definition, but it gives a satisfactory estimation of the reliability of the numerical results among a set of data points. It is only displayed where larger than the symbol used for the data point.

# 2 Viscosity of suspensions as a function of concentration

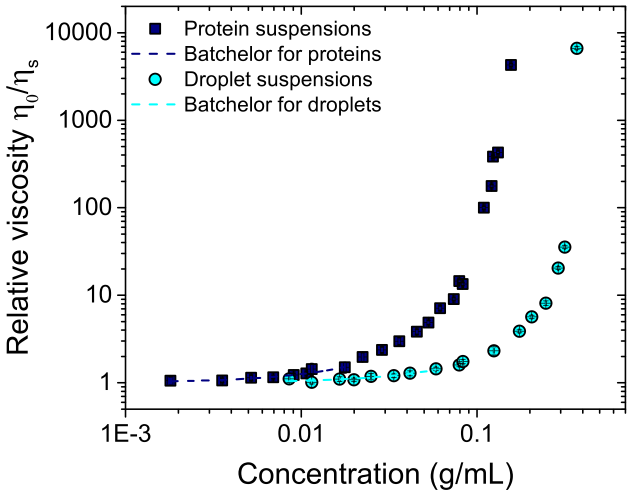


Figure S 1: Viscosity of suspensions as a function of the concentration (in $\mathrm{g\,mL^{-1}}$). Suspensions of: sodium caseinate (□, navy), and sodium caseinate-stabilised nano-sized droplets (◯, cyan).

# 3 Asymptotic behaviour of the modified Quemada model for the viscosity of soft colloidal particles (Equation 5 in the main text)

The semi-empirical viscosity model for soft colloidal particles is based on Quemada model and expressed by:

$$\frac{\eta_0}{\eta_s} = \left(1 - \frac{\phi}{\phi_m^*}\right)^{-2} \tag{2}$$

Where:

$$\phi_m^* = \phi_m \left(1 + \left(\frac{\phi}{\phi_m}\right)^n\right)^{1/n}$$

For $\phi > \phi_m$, it is possible to use limited developments of ln and exp to simplify Equation 2 as follows:

$$
\begin{aligned}
\phi_m^* &= \phi\left(1+\left(\frac{\phi_m}{\phi}\right)^n\right)^{1/n} \\
&= \phi\times\exp\left(\frac{1}{n}\ln\left(1+\frac{\phi_m}{\phi}\right)^n\right) \\
&\approx \phi\times\exp\left(\frac{1}{n}\left(\frac{\phi_m}{\phi}\right)^n\right) \\
\phi_m^* &\approx \phi\times\left(1+\frac{1}{n}\left(\frac{\phi_m}{\phi}\right)^n\right) \qquad (3)
\end{aligned}
$$

This result allows the determination of the slant asymptote of the viscosity at high concentration, since it varies with the power-law:

$$\frac{\eta_0}{\eta_s}(\phi) \propto \phi^{2n} \qquad (4)$$

## 4 Flow curves of suspensions

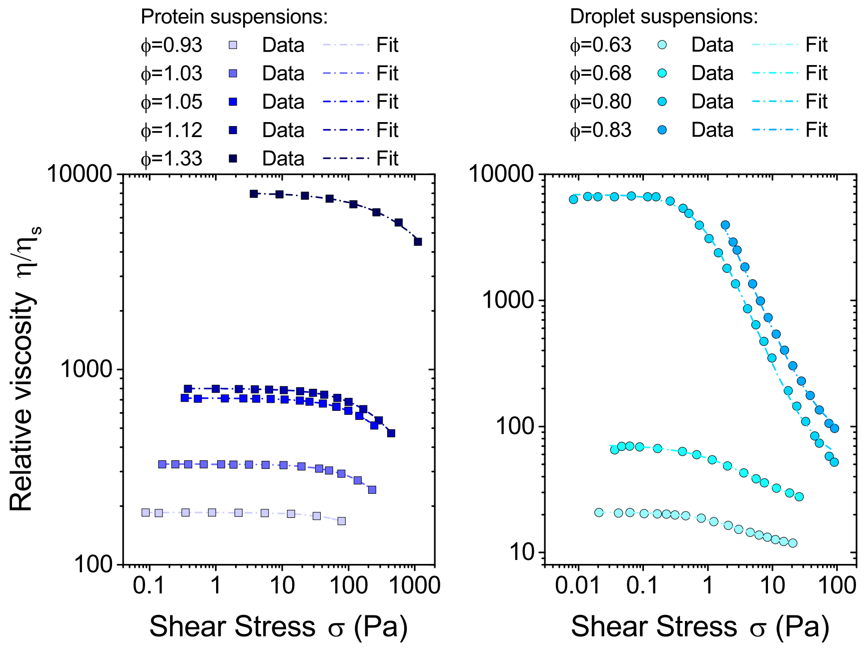


Figure S 2: Flow curves of shear-thinning samples, fitted using the modified Cross equation. The relative viscosity $\eta/\eta_s$ is plotted as a function of the shear stress $\sigma$.
Left (□): Concentrated suspensions of sodium caseinate at effective volume fractions $\phi_{eff,prot}$ of 0.93, 1.03, 1.05, 1.12 and 1.33.
Right (○): Concentrated suspensions of pure sodium caseinate-stabilised oil droplets at effective volume fractions $\phi_{eff,drop}$ of 0.63, 0.68, 0.80 and 0.83. For clarity, only 1/3 of datapoints are displayed for each curve.

# 5 Contributions to the viscosity of the continuous and dispersed phases in mixtures of droplets and proteins

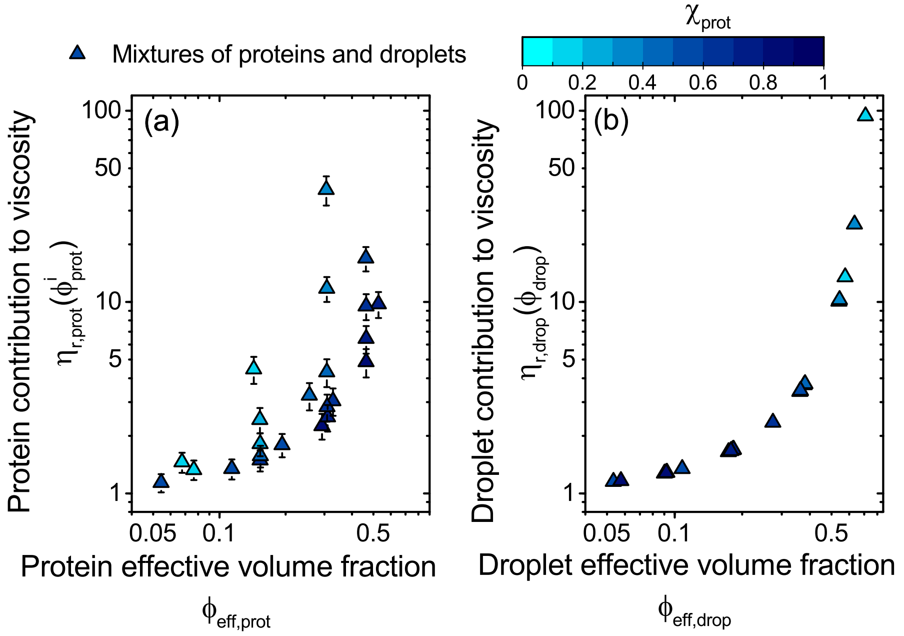


Figure S 3: Relative contributions of the continuous phase and of the dispersed phase alone to the viscosity of caseinate-stabilised emulsions.
(a) Relative viscosity of the continuous phase containing un-adsorbed sodium caseinate aggregates. It is estimated by calculating, for each composition, the volume fraction of protein in the interstices between the droplets $\phi^i_{prot}$. Then the relative viscosity of a suspension of protein at this volume fraction $\eta_{r,prot}\left(\phi^i_{prot}\right)$ is calculated.
(b) Relative viscosity of sodium caseinate-stabilised droplets $\eta_{r,drop}\left(\phi_{drop}\right)$, calculated from the composition of each mixture.
For the two graphs, the colour coding indicates the compositional index of the mixtures $\chi_{prot} = \frac{\phi_{eff,prot}}{\phi_{eff,prot}+\phi_{eff,drop}}$. The error bars are calculated using the error propagation theory (see below), and only displayed if larger than the symbol size.

The contributions of the components of the emulsion to the viscosity are different in the case of the continuous phase (a) and of the dispersed phase (b).

For the continuous phase, containing un-adsorbed proteins, at low concentration, the viscosity hardly depends from the composition of the mixture. But

at higher concentrations, there is a discrepancy of the viscosity of the continuous phase, at a given protein content, with the composition. Indeed, for mixtures with a high droplet content, the concentration of protein in the continuous phase is much higher than for mixtures at low protein content.

In contrast, for the dispersed phase, the viscosity depends only on the droplet content and not on the relative composition of the mixtures.
